# Supplementary material for: Casimir Momentum of a Chiral Molecule in a Magnetic Field
Source: arXiv:1304.6767 source file (2013-10-09)
Supplement: Supplementary file 1 [file Suppl_Mat_LD14704Donaire.pdf]

# Supplemental material: Casimir Momentum of a Chiral Molecule in a Magnetic Field

M. Donaire,[1,2] B.A. van Tiggelen,[1] and G.L.J.A. Rikken[2]

[1] *Université Grenoble 1/CNRS, LPMMC UMR 5493, B.P. 166, 38042 Grenoble, France*
[2] *LNCMI, UPR 3228 CNRS/INSA/UJF Grenoble 1/UPS, Toulouse & Grenoble, France*

In the Letter we compute the Casimir momentum in the asymptotically stationary situation in which the molecule is in its ground state at constant kinetic momentum, $\mathbf{Q}_0$, and at constant magnetic field, $\mathbf{B}_0$. Furthermore, it is mentioned that *for nonrelativistic velocities, terms which depend on the kinetic momentum, $\mathbf{Q}_0$, are negligible in the computation of $\langle\mathbf{P}^{Cas}\rangle$ except for divergent mass renormalization terms that can be made disappear.* It is the purpose of this supplemental material to prove this assertion.

## CALCULATION OF $\langle\mathbf{P}_{\parallel}^{\mathrm{Cas}}\rangle$ FOR NON-ZERO $\mathbf{Q}_0$

For a non-zero value of $\mathbf{Q}_0$, Eq.(9) in the Letter for the longitudinal Casimir momentum reads [0],

$$\langle\mathbf{P}_{\parallel}^{\mathrm{Cas}}\rangle = \sum_{\mathbf{Q},I,\gamma_{\mathbf{k}\epsilon}} \frac{\langle\mathbf{Q}_0,\tilde{\Omega}_0|e\Delta\mathbf{A}|\mathbf{Q},I,\gamma\rangle\langle\mathbf{Q},I,\gamma|\tilde{W}|\mathbf{Q}_0,\tilde{\Omega}_0\rangle}{\mathbf{Q}_0^2/2M+E_0-E_{Q,I,k}} + c.c., \tag{SM1}$$

where $|\mathbf{Q}_0,\tilde{\Omega}_0\rangle = \exp\left(i\mathbf{Q}_0\cdot\mathbf{R}/\hbar\right)|\tilde{\Omega}_0\rangle$, $\Delta\mathbf{A}=\mathbf{A}(\mathbf{r}_N)-\mathbf{A}(\mathbf{r}_e)$, $|\tilde{\Omega}_0\rangle$ is given in Eq.(7), $\tilde{W}$ is given in Eq.(8) and the notation is that explained in the Letter after Eq.(9). We notice from the expression of $\tilde{W}$ in Eq.(8) that $\tilde{W}|\mathbf{Q}_0,\tilde{\Omega}_0\rangle$ in Eq.(SM1) generates a term proportional to $\mathbf{Q}_0$. Therefore, $\langle\mathbf{P}^{\mathrm{Cas}}\rangle$ in priciple depends on $\mathbf{Q}_0$. Using Eqs.(8) and (10), transforming the sums over $\mathbf{Q}$ and $\mathbf{k}$ into continuum integrals and summing over polarization states we arrive at,

$$\begin{aligned}\langle\mathbf{P}_{\parallel}^{\mathrm{Cas}}\rangle &= \frac{-\hbar e^2}{c\epsilon_0 m_e}\int\frac{\mathrm{d}^3k}{(2\pi)^3k}\langle\mathbf{Q}_0,\tilde{\Omega}_0|\frac{(\mathbb{I}-\frac{\mathbf{k}\otimes\mathbf{k}}{k^2})\cdot}{E_k^e+\hbar\mathbf{k}\cdot\mathbf{p}/m_e-\hbar\mathbf{k}\cdot\mathbf{Q}_0/M+H^{HO}+V_C+V_Z-E_0}\\ &\times\ [\mathbf{p}-\frac{m_e}{M}\mathbf{Q}_0+\frac{e}{2}\mathbf{B}_0\wedge\mathbf{r}]|\mathbf{Q}_0,\tilde{\Omega}_0\rangle + c.c.\\ &+\ \frac{\hbar e^2}{c\epsilon_0 m_e}\int\frac{\mathrm{d}^3k}{(2\pi)^3k}\langle\mathbf{Q}_0,\tilde{\Omega}_0|\frac{(\mathbb{I}-\frac{\mathbf{k}\otimes\mathbf{k}}{k^2})\cdot}{E_k^N-\hbar\mathbf{k}\cdot\mathbf{p}/m_N-\hbar\mathbf{k}\cdot\mathbf{Q}_0/M+H^{HO}+V_C+V_Z-E_0}\\ &\times\ [\mathbf{p}+\frac{m_N}{M}\mathbf{Q}_0-\frac{e}{2}\mathbf{B}_0\wedge\mathbf{r}]|\mathbf{Q}_0,\tilde{\Omega}_0\rangle + c.c.\end{aligned} \tag{SM2}$$

The two terms correspond to the diagrams of Fig. 1 and subdominant terms have been omitted. In this expression, $E_k^{e,N}=\hbar^2k^2/2m_{e,N}+\hbar ck$ and the terms $\pm\hbar\mathbf{k}\cdot\mathbf{p}/m_{e,N}$ and $-\hbar\mathbf{k}\cdot\mathbf{Q}_0/M$ stem for the Doppler shifts in the energy of photons of momentum $\hbar\mathbf{k}$ due to the relative motion of the electron and the ion and to the motion of the center of mass as a whole, respectively. After averaging the result of the above integrals over orientations we obtain a series of terms proportional either to $\mathbf{Q}_0$ or to $\mathbf{B}_0$. We will write $\langle\mathbf{P}_{\parallel}^{\mathrm{Cas}}\rangle_{rot}=F\,\mathbf{Q}_0+eG\mathbf{B}_0$, where $F$ and $G$ are functions of $\mathbf{Q}_0$ and $\mathbf{B}_0$. Expanding the energy in the denominators of Eq.(SM3) in powers of Doppler shift factors around $E_k^{e,N}+H^{HO}-E_0$ we obtain,

$$F=\frac{4\hbar^2\alpha}{3\pi M}\int_0^\infty k\mathrm{d}k\left[\frac{1}{E_k^e}+\frac{1}{E_k^N}\right]+\frac{4\alpha}{15\pi}\frac{\mathbf{Q}_0^2}{M^2c^2}+\mathcal{O}\left(\frac{eg_{\parallel}\mathrm{B}_0\mathbf{Q}_0}{M^2c^2}\frac{\hbar\omega_0}{\mu^*c^2}\right)+\mathrm{H.O.T.}, \tag{SM3}$$

$$G=eg_{\parallel}+\mathcal{O}\left(\frac{eg_{\parallel}\mathbf{Q}_0^2}{M^2c^2}\frac{\hbar\omega_0}{\mu^*c^2}\right)+\mathrm{H.O.T.}, \tag{SM4}$$

where H.O.T. stands for *higher order terms*, $\omega_0=(\omega_x+\omega_y+\omega_z)/3$ and $g_{\parallel}=[2\alpha\beta(0)/9\pi\alpha_E(0)]\ln\left(m_e/m_N\right)$, with the ratio between the polarizabilities given by Eq.(17) in the Letter.

---

[0] In these notes we restrict ourselves to the evaluation of the longitudinal momentum. Similar conclusions apply to the transverse momentum terms except for the absence there of divergent mass renormalization terms.

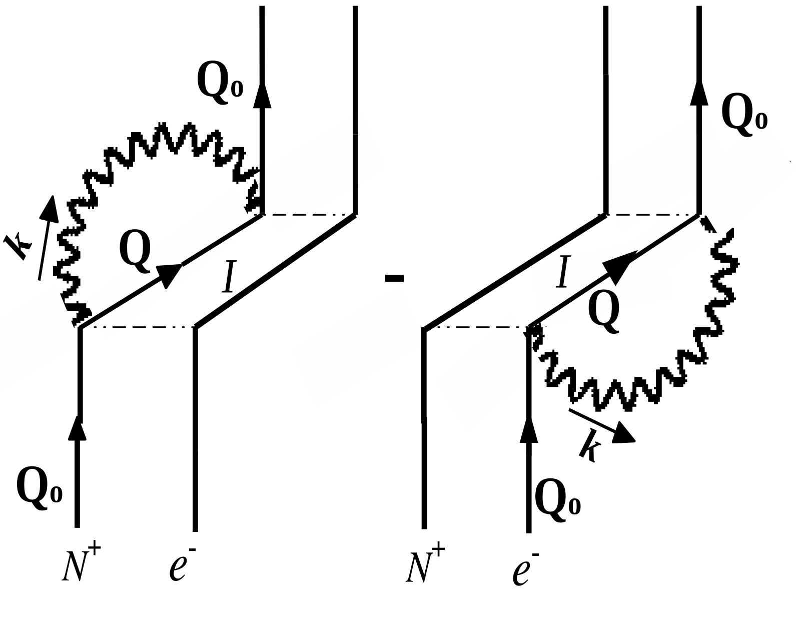


FIG. 1: Feynman diagrams of the processes contributing to $\langle \mathbf{P}_{\parallel}^{\rm Cas}\rangle$ in Eq.(SM2). Note their similarity with the Lamb-shift diagram, except for the fact that here radiative corrections, both to the electron and to the ion momenta, contribute at the same order and with opposite sign.

The terms of Eq.(SM3) for $F$ are obtained in the following way. The first term on the r.h.s. of Eq.(SM3) is a diverging integral that can be made disappear by mass regularization –cf. Refs.[6,7] and below. It comes from the terms $m_{e,N}\mathbf{Q}_0/M$ within the integrands of Eq.(SM2), neglecting all the Doppler shifts and the potentials $V_C+V_Z$ in the denominators there. Note that the terms $\mathbf{p}$ and $e\mathbf{B}_0\wedge\mathbf{r}/2$ in the integrand yield null contribution at the same order of approximation. This is the reason why, for $\mathbf{Q}_0=\mathbf{0}$, no divergent terms show up in Eq.(12) of the Letter. The second term on the r.h.s. comes from the terms $m_{e,N}\mathbf{Q}_0/M$ in the integrands of Eq.(SM2) in combination with a Doppler shift factor $\hbar^2(\mathbf{k}\cdot\mathbf{Q}_0)^2/M^2$ coming from the expansion of the denominators. The third term comes from the terms $m_{e,N}\mathbf{Q}_0/M$ within the integrands of Eq.(SM2) in combination with Doppler shift factors $\hbar^2(\mathbf{k}\cdot\mathbf{Q}_0)(\mathbf{k}\cdot\mathbf{p})/Mm_{e,N}$.

The terms of Eq.(SM4) for $G$ are obtained as follows. The first term on the r.h.s. of Eq.(SM4) is the one found in the Letter. It comes in this case from the application of the terms $\mathbf{p}$ within the integrands of Eq.(SM2), ignoring any Doppler shift but keeping the terms of order $\mathbf{B}_0$. The second term on the r.h.s. is the correction to the first term due to Doppler shift factors $\hbar^2(\mathbf{k}\cdot\mathbf{Q}_0)^2/M^2$ coming from the expansion of the denominators.

## NEGLECT OF $\mathbf{Q}_0$-DEPENDENT TERMS AND MASS RENORMALIZATION PROCEDURE

The two constant terms in the integrand of the divergent integral of Eq.(SM3) differ just by the masses in the energies $E_k^e$ and $E_k^N$, and do not depend on the binding energy of the electron-ion system. Therefore, they correspond to radiative corrections to the masses of the free particles. Both together amount to a divergent mass shift,

$$\Delta M=\frac{4\hbar^2\alpha}{3\pi}\int_0^\infty k\mathrm{d}k\left[\frac{1}{E_k^e}+\frac{1}{E_k^N}\right], \qquad \text{(SM5)}$$

which can be absorbed into the definition of the physical mass ($phys$) [6,7], $M_{phys}=M+\Delta M$.

The rest of terms in $F$ are several orders of magnitude smaller than unity for a non-relativistic momentum $\mathbf{Q}_0$. In particular, for a molecule starting at rest at zero magnetic field, the final kinetic momentum and also $eg_{\parallel}\mathrm{B}_0$ were found to be of the order of $10^{-34}$ kg m/s for $\mathrm{B}_0$ =10 T, while $M_{phys}c\sim10^{-19}$kg m/s. In the same manner for $G$, the second term on the r.h.s. of Eq.(SM4) is even smaller with respect to the first one because of the additional factor $\hbar\omega_0/\mu^*c^2\sim10^{-13}$. Therefore, we can write in good approximation $\langle\mathbf{P}_{\parallel}^{\rm Cas}\rangle_{rot}=eg_{\parallel}\mathbf{B}_0+(\Delta M/M)\mathbf{Q}_0$, which shows that, except for the mass renormalization term, the calculation of $\langle\mathbf{P}_{\parallel}^{\rm Cas}\rangle$ is independent of $\mathbf{Q}_0$.

Further, including the contribution of the transverse momentum, $\langle\mathbf{P}_{\perp}^{\rm Cas}\rangle_{rot}=eg_{\perp}\mathbf{B}_0$, with $g_{\perp}=-2\alpha\beta(0)/9\pi\alpha_E(0)$, and as a result of Eq.(5) we end up with $(1+\Delta M/M)\mathbf{Q}_0=-eg\mathbf{B}_0$, where $g=g_{\parallel}+g_{\perp}$. Equivalently, the relation

between $\mathbf{Q}_0$ and $\mathbf{B}_0$ can be written as $\langle M_{phys}\dot{\mathbf{R}}\rangle = -eg\mathbf{B}_0$, which shows that $\Delta M$ is indeed a mass renormalization term.
